# Supplementary material for: Spreading dynamics of droplets impacting on oscillating hydrophobic substrates
Source: arXiv:2306.10688 ancillary file (2023-06-19)
Supplement: Supplementary file 1 [file SM_Potnis_Saha_JFM.pdf]

# Supplementary Material: *Spreading dynamics of droplets impacted on oscillating substrates* by A. Potnis and A. Saha

## 1 Effect of impact parameters on maximum spreading

### 1.1 Effect of amplitude:

The effect of the amplitude of oscillation on the spreading behavior was assessed by maintaining a constant frequency of oscillation ($f$) and varying the amplitude ($A$) of oscillation as a function of phase ($\phi$). The variation in $D^*_{max}/D_{max,s}$ for a range of amplitudes are shown in Fig. 1a and b, for frequencies 100 $Hz$ and 200 $Hz$ respectively. The impact $We(= 27)$ and $Re(= 2300)$ were kept constant. The corresponding time for attaining these maximum spreads ($t_{max}/t_{max,s}$) are plotted in Fig. 2a and b.

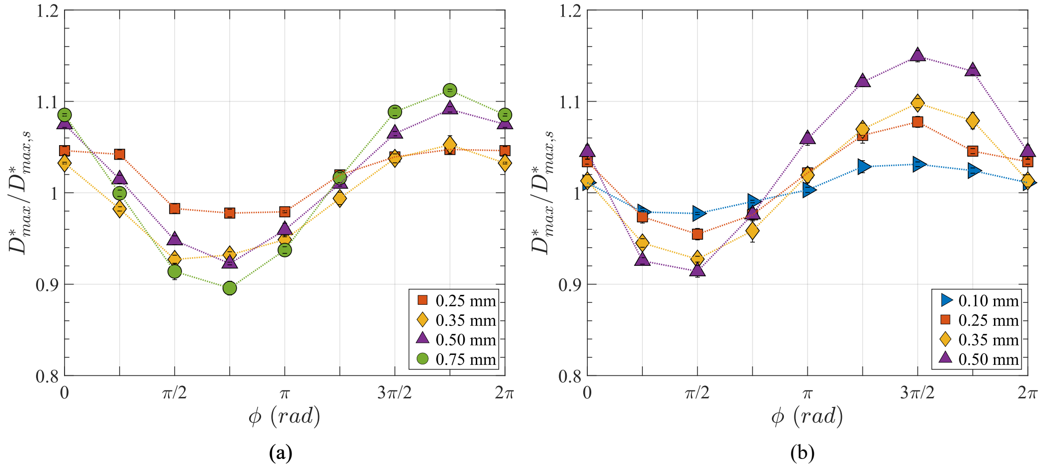


Figure 1: Normalized maximum spread, $D^*_{max}/D^*_{max,s}$ as a function of phase, $\phi$ at impact for various oscillation amplitudes. (a) 100 $Hz$ (b) 220 $Hz$. Here the error bars represent the extent of standard deviation about the mean value.

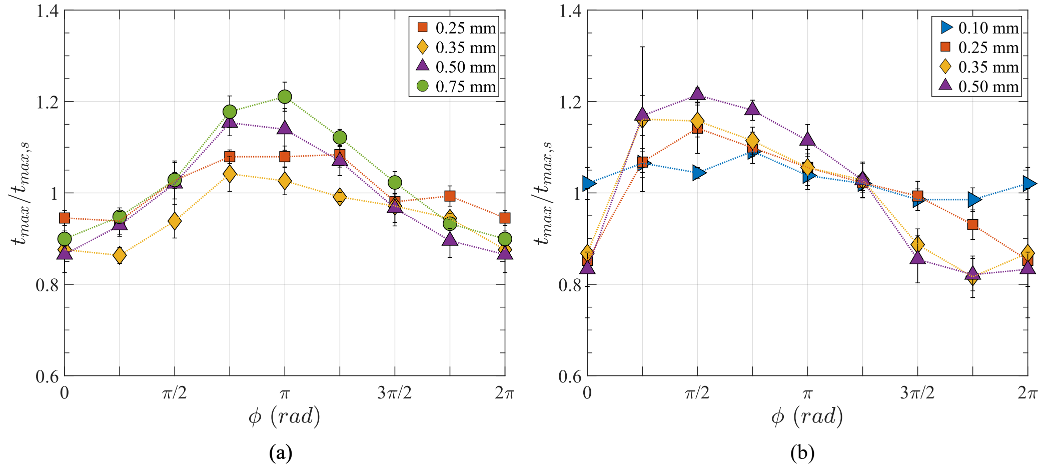


Figure 2: Normalized time to maximum spread, $t_{max}/t_{max,s}$ as a function of phase, $\phi$ at impact for various oscillation amplitudes. (a) 100 $Hz$ (b) 220 $Hz$. Here the error bars represent the extent of standard deviation about the mean value.

## 1.2 Effect of Weber number

$We$ was varied by controlling the impact velocity of the droplet ($V_0$). The frequency and amplitude were held constant, and for each $We$ investigated $(27, 44$ & $77)$, the phase at impact was varied. This was repeated for two frequencies, 100 $Hz$ and 220 $Hz$. The amplitude of oscillation was set at $A = 0.25$ $mm$. Figure 3 presents the maximum spread during impact on oscillating substrates, normalized by corresponding value for impact on the impact on the static substrate ($D^*_{max}/D^*_{max,s}$). Figure 4 shows the normalized time $t_{max}/t_{max,s}$ for maximum spreading diameter.

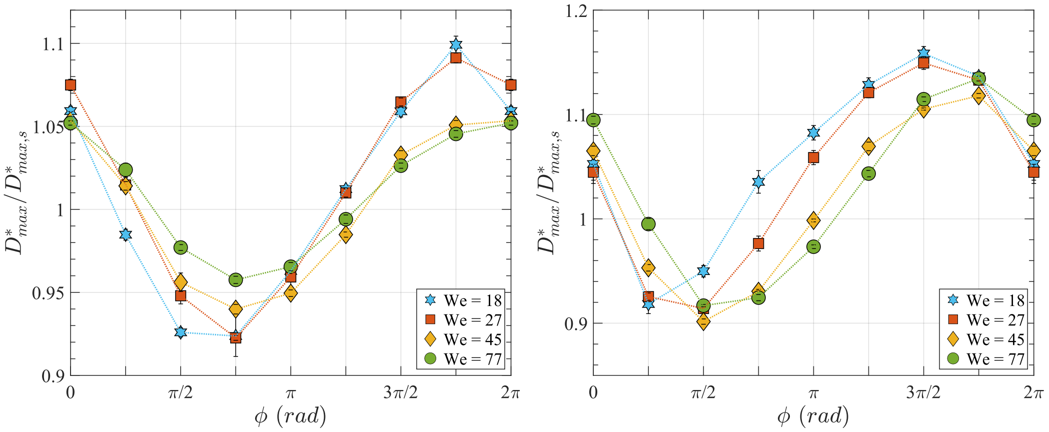


(a) (b)

Figure 3: Normalized maximum spread, $D^*_{max}/D^*_{max,s}$ as a function of phase, $\phi$ at impact for various Weber numbers $We = 18, 27, 45$ & $77$ for (a) $f = 100$ $Hz$ (b) $f = 220$ $Hz$. Here the error bars represent the extent of standard deviation about the mean value.

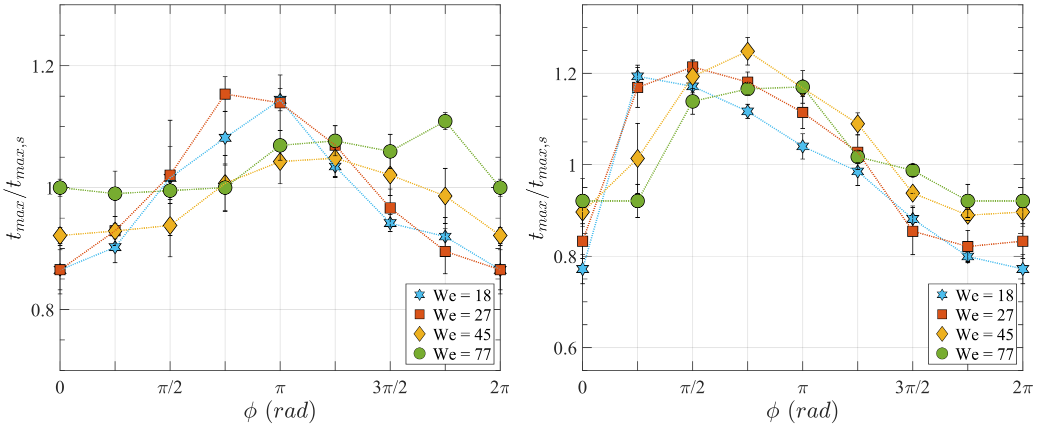


(a) (b)

Figure 4: Normalized time to maximum spread, $t_{max}/t_{max,s}$ as a function of phase, $\phi$ at impact for various Weber numbers $We = 18, 27, 45$ & $77$ for (a) $f = 100$ $Hz$ (b) $f = 220$ $Hz$. Here the error bars represent the extent of standard deviation about the mean value.

Figure 5 shows the one frequency for each $We$ studied, for which *Stage-II* spreading was observed (at amplitude $A = 0.25$ $mm$). The $\phi$ for which *Stage-II* spread occurs is $\pi/2$ and $5\pi/4$ as identified by the increased value of $t_{max}/t_{max,s}$ in Fig. 5b.

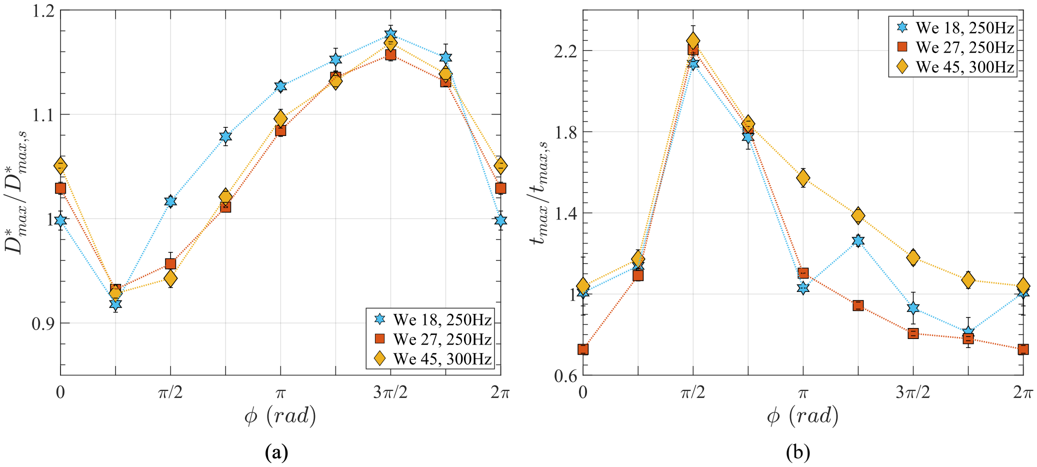


Figure 5: Second stage spreading at lowest frequencies observed for various Weber numbers $We = 18, 27$, & 45 a) Normalized maximum spread, $D^*_{max}/D^*_{max,s}$ as a function of phase, $\phi$ at impact b) Normalized time to maximum spread, $t_{max}/t_{max,s}$ as a function of phase, $\phi$ at impact. Here the error bars represent the extent of standard deviation about the mean value.

## 2 Evolution of top of falling droplet

Here, we compare the trajectory of the tip of the impacting droplet and the instantaneous droplet spread obtained from experiments. The dashed black line shows the trajectory of a motion with constant velocity $V_0$. It can be seen that for most of its trajectory, the tip of the droplet closely follows this line. Thus, it supports the assumption of constant velocity ($V = V_0$) for the tip of the droplet till $t = \tau$ used in the theoretical estimation of $\tau$ (Sec. 4.1.2).

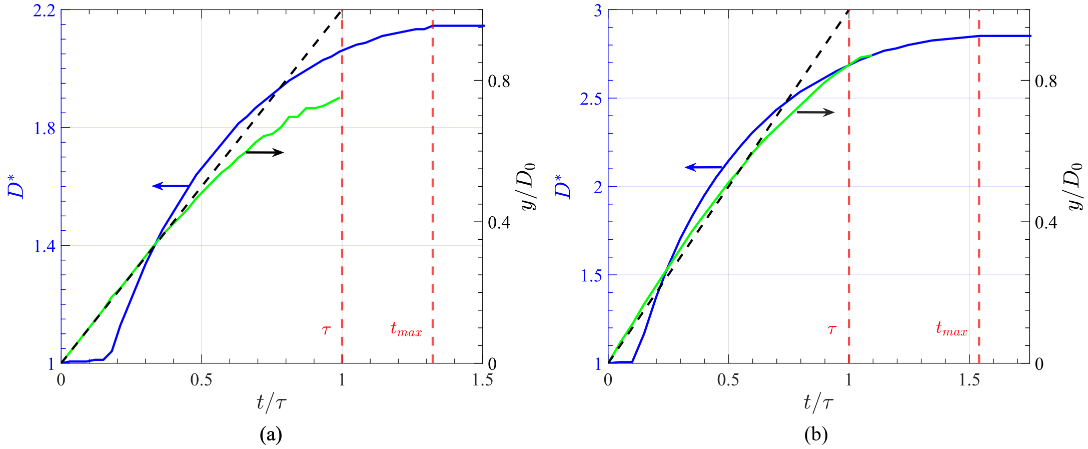


Figure 6: Temporal evolution of post-impact normalized droplet diameter (D$^*$) along with the trajectory of displacement of the top of falling droplet for (a) Static impact $We = 27$ (b) Oscillating substrate at $We = 77$ with f $= 220\ Hz$, A $= 0.25mm$ and $\phi = \pi/4\ rad$; The black dashed lines ($--$) show the displacement at constant $V = V_0$. Red dashed lines ($--$) highlight the 'crashing time' ($\tau$) and the time to maximum spread (t$_{max}$).

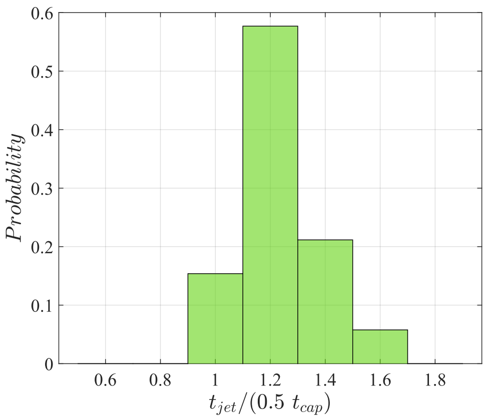


Figure 7: Relative probability of experimentally observed jetting time normalized with respect to estimated jetting time ($0.5\ t_{cap}$) for a representative set of data including a wide range of $f$, $A$, $\phi$, and $We$.

# 3 Time for post-impact capillary jetting

Figure 7 shows the probability of experimentally observed time for jetting after impact ($t_{jet}$), normalized by $0.5\ t_{cap}$, for a representative set of data covering all the frequency ($f$), amplitude ($A$), the phase at impact ($\phi$), and Weber number ($We$). Here $t_{cap} = \sqrt{\rho D_0^3/\gamma}$ is the capillary time. The figure shows that jetting occurs at $\approx (1/2)t_{cap}$ irrespective of impact or oscillation parameters.
